# Supplementary material for: Efficient Conformal Prediction via Cascaded Inference with Expanded Admission
Source: arXiv:2007.03114 source file (2021-02-02)
Supplement: Supplementary file 1 [file cascaded_predictive_eff.tex]

\subsection{Cascaded CP and predictive efficiency}
Our cascaded pipeline allows for the combination of multiple measures, some of which are computationally expensive. Figure~\ref{fig:ecdf-cascade} shows the contribution of each layer to the final efficiency. For example, in the IR task, the BM25 CP already drastically trims the set of candidates by 90\%, on average. The stronger neural classifier is then only needed on a fraction of the candidate space---and can be used to further reject more than $2/3$rds of the remaining predictions, all while still preserving equivalent coverage. Note that, at times, the full cascade can remarkably lead to an ultimately \underline{more} powerful predictor than even just using the strongest individual measure over all labels (which is also computationally inefficient)---see IR in Figure~\ref{fig:ecdf-eps-min}  for a positive example. This depends, however, in how complementary the nonconformity measures are. In DR, \emph{chemprop} does provide much performance gains over RF on our tested data. Therefore, and due to some disagreements between the models and the effect of the MHT correction, the cascade increases the predictive efficiency. In QA, even though the CLS logit alone provides a strong classifier by itself (though computationally expensive), the cascade can improve slightly further.
% This depends on how complementary the nonconformity measures are (e.g., in QA the metrics are highly correlated and therefore lead to better \emph{computational} efficiency, but similar \emph{predictive} efficiency). It also depends on the size of the calibration set, and its effect on the MHT correction (e.g., in DR the small sample size reduces the effectiveness of the ECDF correction, and makes the combination more conservative than using the nonconformity measures individually).

% The main goal of our cascaded pipeline is to allow for the combination of multiple classifiers, some of which are computationally expensive. Figure~\ref{fig:ecdf-cascade} shows that this cascade indeed leads to an improved CP with smaller prediction sets in general. For example, in the IR task in Figure~\ref{fig:ecdf-cascade} (b), the BM25 CP already drastically trims the set of candidates by 90.5\%, on average. The stronger neural classifier is then only needed on a fraction of the candidate space---and can be used to further reject more than $2/3$rds of the remaining predictions, all while still preserving equivalent coverage.

\begin{figure}[h]
\centering
\begin{subfigure}{0.32\textwidth}
\includegraphics[width=1.05\linewidth]{figures/sample/test/simes/qa/eps_eff_break.png} 
\vspace*{-1.8\baselineskip}
\caption{QA}
\end{subfigure}
~
\begin{subfigure}{0.32\textwidth}
\includegraphics[width=1.05\linewidth]{figures/sample/test/ecdf/ir/eps_eff_break.png}
\vspace*{-1.8\baselineskip}
\caption{IR}
\end{subfigure}
~
\begin{subfigure}{0.32\textwidth}
\includegraphics[width=1.05\linewidth]{figures/sample/test/simes/hiv/eps_eff_break.png} 
\vspace*{-1.8\baselineskip}
\caption{DR}
\end{subfigure}
\small
\vspace{-5pt}
\caption{\emph{How does cascading multiple nonconformity measures (\S\ref{sec:combination}) affect the predictive efficiency?} We observe that the first level typically greatly reduces the label space, while the subsequent levels then typically substantially improve the efficiency (QA, IR). In the DR task we observe a negative result, where the small sample size (the $n$ in $\cset$) causes the MHT-corrected CP to be too conservative. Surprisingly, on the test data, the cheaper RF measure on its own actually outperforms \texttt{chemprop}.}
\label{fig:ecdf-cascade}
\vspace{-19pt}
\end{figure}
